# Supplementary material for: Hybrid Beamforming for Millimeter Wave Full-Duplex under Limited Receive Dynamic Range
Source: arXiv:2012.11647 source file (2020-12-21)
Supplement: Supplementary file 1 [file sec-appendix.tex]

\appendices

% \section{Reformulating \eqref{eq:opt-sat} for Semidefinite Programming} \label{app:reformulating}

%\section{Proof of Induced Infinity Norm Property} \label{app:norm-inf-proof}
%
%Let us assume $\ev{\vx \vx\ctrans} = \frac{1}{N} \mI$.
%The inequality
%\begin{align}
%\norminf{\mA \vx}^2 \leq P
%\end{align}
%can be equivalently written as
%\begin{align}
%\diag{\mA \vx \vx\ctrans \mA\ctrans} \leq P \cdot \vone
%\end{align}
%Then, taking an expectation over $\vx$ gives us
%\begin{align}
%\ev{\diag{\mA \vx \vx\ctrans \mA\ctrans}} &\leq P \cdot \vone \\
%\diag{\mA \ev{\vx \vx\ctrans} \mA\ctrans} &\leq P \cdot \vone \\
%\frac{1}{N} \diag{\mA \mA\ctrans} &\leq P \cdot \vone \\
%\frac{1}{N} \norminf{\mA}^2 &\leq P
%\end{align}

% \pagebreak

\section{Quantization Properties and Derivations}

\subsection{Preliminaries}
We assume a uniform, mid-riser quantizer.

\subsection{Quantization Level Size, $q$}
We assume gain control adjusts the input signal amplitude according to the signal's average power at the \adc input. 
We represent this equivalently by adjusting the input range of the \adc to fit the signal rather than adjusting the signal to fit the input range.
Having assumed uniform quantization, we are interested in the quantization level size $q$ (i.e., distance between levels in volts) for a signal with average power $P$.
To map between average power and voltage, we require some assumption on the waveform statistics.
As such, we assume the signal at the \adc input to be approximately sinusoidal, solely for the sake of deriving an expression for $q$.

With $b$ bits of resolution, we have $L=2^b$ quantization levels spread out over the \adc input range.
If the peak-to-peak voltage of the \adc input is $\Vpkpk$, the quantization level size is simply
\begin{align}
q = \frac{\Vpkpk}{L}
\end{align}
Having assumed a sinusoidal input, we note that the peak-to-peak voltage is twice the peak voltage
\begin{align}
q = \frac{2\Vpk}{L}
\end{align}
A sinusoid with power $P$ has a peak voltage of
\begin{align}
\Vpk = \sqrt{2} \cdot \Vrms = \sqrt{2} \cdot \sqrt{P}
\end{align}
which leads directly to
\begin{align}
q = \frac{2 \sqrt{2} \cdot \sqrt{P}}{L}
\end{align}
and for convenience
\begin{align}
q^2 = \frac{8 \cdot P}{2^{2b}}
\end{align}

\subsection{Quantization Noise Power, $\powerquant$}
We assume quantization noise is uniform between quantization levels.
\begin{align}
\powerquant 
&= \var{\equant} \\
&= \int_{-\infty}^{\infty} e^2 \cdot \pdf{\equant}{e} \ \dde \\
&= \int_{-q/2}^{q/2} e^2 \cdot \frac{1}{q} \ \dde \\
&= 2 \times \frac{(q/2)^3}{3q} \\
&= \frac{q^2}{12}
\end{align}

\subsection{Maximum Allowed Self-Interference Power, $\powersimaxadc$}
\begin{align}
\snrdesout &= \deltasnrdes \cdot \snrdesin \\
\frac{\powerdesadc}{\powernoiseadc + \powerquant} &= \deltasnrdes \cdot \snrdesin \\
\frac{1}{\frac{\powernoiseadc}{\powerdesadc} + \frac{\powerquant}{\powerdesadc}} &= \deltasnrdes \cdot \snrdesin \\
{\frac{1}{\snrdesin} + \frac{\powerquant}{\powerdesadc}} &= \frac{1}{\deltasnrdes \cdot \snrdesin} \\
\frac{\powerquant}{\powerdesadc} &= \frac{1}{\snrdesin} \cdot \frac{1-\deltasnrdes}{\deltasnrdes} \\
{\frac{8 \cdot \parens{\powerdesadc + \powersiadc + \powernoiseadc} \cdot \adcbackoff}{2^{2\adcbits} \cdot 12 }} &= \frac{\powerdesadc}{\snrdesin} \cdot \frac{1-\deltasnrdes}{\deltasnrdes} \\
\parens{\powerdesadc + \powersiadc + \powernoiseadc} \cdot \adcbackoff &= \frac{\powerdesadc}{\snrdesin} \cdot 2^{2\adcbits} \cdot 1.5  \cdot \frac{1-\deltasnrdes}{\deltasnrdes}
\end{align}
which leads to
\begin{align}
\powersiadc  &= \frac{\powerdesadc}{\adcbackoff \cdot \snrdesin} \cdot 2^{2\adcbits} \cdot 1.5  \cdot \frac{1-\deltasnrdes}{\deltasnrdes} - \powerdesadc - \powernoiseadc \\
\powersiadc  &= \powernoiseadc \parens{ \frac{2^{2\adcbits} \cdot 1.5}{\adcbackoff}  \cdot \frac{1-\deltasnrdes}{\deltasnrdes} - \snrdesin - 1 }
\end{align}
need to replace this with $\powersimaxadc$.

% \section{Alternate Forms of \eqref{eq:problem-inner}}

\input{sec-mse.tex}
