# Supplementary material for: Hybrid Beamforming for Millimeter Wave Full-Duplex under Limited Receive Dynamic Range
Source: arXiv:2012.11647 source file (2020-12-21)
Supplement: Supplementary file 2 [file eq-si-channel-los.tex]

\begin{align} \label{eq:si-channel-los}
	\left[\channel^{\textrm{NF}}_{ii}\right]_{v,u} &= \frac{\gamma}{r_{u,v}}\exp \left(-\j 2 \pi \frac{r_{u,v}}{\lambda} \right)
\end{align}
