# Supplementary material for: Hybrid Beamforming for Millimeter Wave Full-Duplex under Limited Receive Dynamic Range
Source: arXiv:2012.11647 source file (2020-12-21)
Supplement: Supplementary file 3 [file eq-si-channel-rice.tex]

\begin{align} \label{eq:si-channel-rice}
	\channel_{ii} &= \sqrt{\frac{\kappa}{\kappa + 1}} \channel^{\mathrm{NF}}_{ii} + \sqrt{\frac{1}{\kappa + 1}} \channel^{\mathrm{FF}}_{ii}
\end{align}
